# Supplementary material for: Interactive Neural Painting
Source: arXiv:2307.16441 source file (2023-07-31)
Supplement: Supplementary file 1 [file sequence.tex]

\begin{table*}[t]
    \centering
    
    \resizebox{\linewidth}{!}{
    \setlength\tabcolsep{0pt}
    \footnotesize
    
    \begin{tabular}{c@{\hskip 0.7mm}ccccccc}
         & $k=1$ & $k=4$ & $K=8$ & $k=12$ & $k=16$ & $k=20$ & $k=24$ \\
            % New sample
            \rotatebox{90}{\hspace{3.5mm}\methodname}  & \includegraphics[trim=2 0 0 2,clip,width=0.2\columnwidth]{supp_mat/oxford/sequence/our/0.jpg} &
            \includegraphics[trim=2 0 0 2,clip,width=0.2\columnwidth]{supp_mat/oxford/sequence/our/4.jpg} &
            \includegraphics[trim=2 0 0 2,clip,width=0.2\columnwidth]{supp_mat/oxford/sequence/our/8.jpg} &
            \includegraphics[trim=2 0 0 2,clip,width=0.2\columnwidth]{supp_mat/oxford/sequence/our/12.jpg} &
            \includegraphics[trim=2 0 0 2,clip,width=0.2\columnwidth]{supp_mat/oxford/sequence/our/16.jpg} &
            \includegraphics[trim=2 0 0 2,clip,width=0.2\columnwidth]{supp_mat/oxford/sequence/our/20.jpg} &
            \includegraphics[trim=2 0 0 2,clip,width=0.2\columnwidth]{supp_mat/oxford/sequence/our/23.jpg} \\
                     
            \rotatebox{90}{\hspace{3.5mm}PT} &\includegraphics[trim=2 0 0 2,clip,width=0.2\columnwidth]{supp_mat/oxford/sequence/pt/0.jpg} &
            \includegraphics[trim=2 0 0 2,clip,width=0.2\columnwidth]{supp_mat/oxford/sequence/pt/4.jpg} &
            \includegraphics[trim=2 0 0 2,clip,width=0.2\columnwidth]{supp_mat/oxford/sequence/pt/8.jpg} &
            \includegraphics[trim=2 0 0 2,clip,width=0.2\columnwidth]{supp_mat/oxford/sequence/pt/12.jpg} &
            \includegraphics[trim=2 0 0 2,clip,width=0.2\columnwidth]{supp_mat/oxford/sequence/pt/16.jpg} &
            \includegraphics[trim=2 0 0 2,clip,width=0.2\columnwidth]{supp_mat/oxford/sequence/pt/20.jpg} &
            \includegraphics[trim=2 0 0 2,clip,width=0.2\columnwidth]{supp_mat/oxford/sequence/pt/23.jpg} \\

            \rotatebox{90}{\hspace{3.5mm}SNP} &\includegraphics[trim=2 0 0 2,clip,width=0.2\columnwidth]{supp_mat/oxford/sequence/snp/0.jpg} &
            \includegraphics[trim=2 0 0 2,clip,width=0.2\columnwidth]{supp_mat/oxford/sequence/snp/4.jpg} &
            \includegraphics[trim=2 0 0 2,clip,width=0.2\columnwidth]{supp_mat/oxford/sequence/snp/8.jpg} &
            \includegraphics[trim=2 0 0 2,clip,width=0.2\columnwidth]{supp_mat/oxford/sequence/snp/12.jpg} &
            \includegraphics[trim=2 0 0 2,clip,width=0.2\columnwidth]{supp_mat/oxford/sequence/snp/16.jpg} &
            \includegraphics[trim=2 0 0 2,clip,width=0.2\columnwidth]{supp_mat/oxford/sequence/snp/20.jpg} &
            \includegraphics[trim=2 0 0 2,clip,width=0.2\columnwidth]{supp_mat/oxford/sequence/snp/23.jpg} \\
            
            \rotatebox{90}{\hspace{3.5mm}SNP+} &\includegraphics[trim=2 0 0 2,clip,width=0.2\columnwidth]{supp_mat/oxford/sequence/snp2/0.jpg} &
            \includegraphics[trim=2 0 0 2,clip,width=0.2\columnwidth]{supp_mat/oxford/sequence/snp2/4.jpg} &
            \includegraphics[trim=2 0 0 2,clip,width=0.2\columnwidth]{supp_mat/oxford/sequence/snp2/8.jpg} &
            \includegraphics[trim=2 0 0 2,clip,width=0.2\columnwidth]{supp_mat/oxford/sequence/snp2/12.jpg} &
            \includegraphics[trim=2 0 0 2,clip,width=0.2\columnwidth]{supp_mat/oxford/sequence/snp2/16.jpg} &
            \includegraphics[trim=2 0 0 2,clip,width=0.2\columnwidth]{supp_mat/oxford/sequence/snp2/20.jpg} &
            \includegraphics[trim=2 0 0 2,clip,width=0.2\columnwidth]{supp_mat/oxford/sequence/snp2/23.jpg} \\
            
            \rotatebox{90}{\hspace{3.5mm}\methodname} &\includegraphics[trim=2 0 0 2,clip,width=0.2\columnwidth]{supp_mat/ade/sequence/our/0.jpg} &
            \includegraphics[trim=2 0 0 2,clip,width=0.2\columnwidth]{supp_mat/ade/sequence/our/4.jpg} &
            \includegraphics[trim=2 0 0 2,clip,width=0.2\columnwidth]{supp_mat/ade/sequence/our/8.jpg} &
            \includegraphics[trim=2 0 0 2,clip,width=0.2\columnwidth]{supp_mat/ade/sequence/our/12.jpg} &
            \includegraphics[trim=2 0 0 2,clip,width=0.2\columnwidth]{supp_mat/ade/sequence/our/16.jpg} &
            \includegraphics[trim=2 0 0 2,clip,width=0.2\columnwidth]{supp_mat/ade/sequence/our/20.jpg} &
            \includegraphics[trim=2 0 0 2,clip,width=0.2\columnwidth]{supp_mat/ade/sequence/our/23.jpg} \\

            \rotatebox{90}{\hspace{4mm}PT} & \includegraphics[trim=2 0 0 2,clip,width=0.2\columnwidth]{supp_mat/ade/sequence/pt/0.jpg} &
            \includegraphics[trim=2 0 0 2,clip,width=0.2\columnwidth]{supp_mat/ade/sequence/pt/4.jpg} &
            \includegraphics[trim=2 0 0 2,clip,width=0.2\columnwidth]{supp_mat/ade/sequence/pt/8.jpg} &
            \includegraphics[trim=2 0 0 2,clip,width=0.2\columnwidth]{supp_mat/ade/sequence/pt/12.jpg} &
            \includegraphics[trim=2 0 0 2,clip,width=0.2\columnwidth]{supp_mat/ade/sequence/pt/16.jpg} &
            \includegraphics[trim=2 0 0 2,clip,width=0.2\columnwidth]{supp_mat/ade/sequence/pt/20.jpg} &
            \includegraphics[trim=2 0 0 2,clip,width=0.2\columnwidth]{supp_mat/ade/sequence/pt/23.jpg} \\

            \rotatebox{90}{\hspace{3.5mm}SNP} &\includegraphics[trim=2 0 0 2,clip,width=0.2\columnwidth]{supp_mat/ade/sequence/snp/0.jpg} &
            \includegraphics[trim=2 0 0 2,clip,width=0.2\columnwidth]{supp_mat/ade/sequence/snp/4.jpg} &
            \includegraphics[trim=2 0 0 2,clip,width=0.2\columnwidth]{supp_mat/ade/sequence/snp/8.jpg} &
            \includegraphics[trim=2 0 0 2,clip,width=0.2\columnwidth]{supp_mat/ade/sequence/snp/12.jpg} &
            \includegraphics[trim=2 0 0 2,clip,width=0.2\columnwidth]{supp_mat/ade/sequence/snp/16.jpg} &
            \includegraphics[trim=2 0 0 2,clip,width=0.2\columnwidth]{supp_mat/ade/sequence/snp/20.jpg} &
            \includegraphics[trim=2 0 0 2,clip,width=0.2\columnwidth]{supp_mat/ade/sequence/snp/23.jpg} \\
            
            \rotatebox{90}{\hspace{3.5mm}SNP+} & \includegraphics[trim=2 0 0 2,clip,width=0.2\columnwidth]{supp_mat/ade/sequence/snp2/0.jpg} &
            \includegraphics[trim=2 0 0 2,clip,width=0.2\columnwidth]{supp_mat/ade/sequence/snp2/4.jpg} &
            \includegraphics[trim=2 0 0 2,clip,width=0.2\columnwidth]{supp_mat/ade/sequence/snp2/8.jpg} &
            \includegraphics[trim=2 0 0 2,clip,width=0.2\columnwidth]{supp_mat/ade/sequence/snp2/12.jpg} &
            \includegraphics[trim=2 0 0 2,clip,width=0.2\columnwidth]{supp_mat/ade/sequence/snp2/16.jpg} &
            \includegraphics[trim=2 0 0 2,clip,width=0.2\columnwidth]{supp_mat/ade/sequence/snp2/20.jpg} &
            \includegraphics[trim=2 0 0 2,clip,width=0.2\columnwidth]{supp_mat/ade/sequence/snp2/23.jpg} \\
        
    \end{tabular}
    }
    \vspace{2mm}
    \captionof{figure}{Visualization of prediction results for a sequence of 24 predicted strokes.}
    \label{fig:sequence}
\end{table*}
