# Supplementary material for: Interactive Neural Painting
Source: arXiv:2307.16441 source file (2023-07-31)
Supplement: Supplementary file 2 [file supp_experiments.tex]

In this Supplementary Material, we provide additional details about dataset acquisition, parametrization and rendering of the strokes (Sec. \ref{sec:supp_dataset}), a description of the architecture and of the losses computation procedure (Sec.~\ref{sec:supp_method}), ablation results on \emph{ADE 20K Outdoor INP} and user study details (Sec.~\ref{sec:supp_experiments}), and additional qualitative results (Sec.~\ref{sec:supp_qualitative}). 

This Supplementary Material is complemented by a supplementary website (See. \href{run:website/index.html}{main.html}) where we show additional qualitative results in the form of videos. In particular, we showcase a demo of \methodname~in an Interactive Neural Painting (INP) scenario, where a user interacts with our model to paint a reference image.

\section{Dataset}
\label{sec:supp_dataset}
Due to the cost associated with the acquisition of a real stroke dataset, we evaluate our model on two synthetic stroke datasets, built to mimic human painting style (see Sec. 4.1 of the main paper for a discussion). Here we detail the dataset acquisition procedure. Examples from the dataset are provided on the supplementary website. \\% (See \href{run:website/datasets.html}{datasets.html}).\\

\noindent \textbf{Images.} We rely on two publicly available datasets, each containing images and associated segmentation masks.
The \textit{Oxford-IIIT Pet} \cite{parkhi2012cats} dataset, contains 7349 images of cats and dogs of different species for a total of 37 different classes. 
The \textit{ADE 20K} \cite{zhou2017ade20k} dataset is a large-scale dataset containing $20,\!100$ images from more than $3K$ classes. The dataset is filtered to contain images of outdoor scenes, resulting in a subset of 5000 images. %Each image is rescaled to a fixed size of $256\times256$ and is decomposed into a sequence of stroke parameters following Stylized Neural Painting \cite{zou2021stylized}.
\\

\noindent \textbf{Strokes Parametrization.} Following the work of Zou \etal \cite{zou2021stylized}, we parametrize the strokes as $s\!=\!(x, \rho, \sigma, \omega)$. The center of the stroke is represented by $x\!=\!(x_x, x_y)$. %, with the coordinates normalized by the canvas size. % such that $x \in [0, 1]$. 
The height and width of the strokes are represented by $\sigma\!=\!(\sigma_h, \sigma_w)$, while $\omega$ represents the orientation, which is the counter-clockwise angle in the range $[0, \pi]$. % and normalized by $\pi$.
Lastly, the color of the stroke is represented by $\rho\!=\!(\rho_r, \rho_g, \rho_b)$.
All the parameters are normalized to lie in the interval $[0, 1]$. \\

\noindent \textbf{Decomposition.}~We make use of Stylized Neural Painting (SNP) \cite{zou2021stylized}, to extract a sequence of brushstrokes from a given image. We notice that SNP tends to produce very large strokes in the first iterations of the method, which cover a wide area of the canvas. This practice is unrealistic since the size limitations of physical brushstrokes would prevent a human painter from doing this. To circumvent such behavior, we clamp the parameter $\sigma$ to a maximum value of $0.4$.
As described in \cite{zou2021stylized}, we employ a progressive rendering pipeline with a total of 4 iterations, dividing the image in a grid with 4, 9, 16, and 25 regions. We allocate a different number of strokes during the progressive rendering process, respectively 30, 20, 15, and 10 to each region, which results in a total of 790 strokes per image. 
Lastly, SNP represents the color of each stroke using two triples of $(\mathrm{r}, \mathrm{g}, \mathrm{b})$ values that are interpolated to obtain a smooth color. For simplicity, we use the average of the two, and represent the stroke with a uniform color $\rho$. \\

\noindent \textbf{Reordering.} We  perform a reordering of the sequences, by minimizing the following cost function, computed along the complete stroke sequence:
 
 \begin{align}
\mathrm{cost} &= \sum_{t=2}^{T} (\lambda^{\mathrm{ord}}_x \left\|x^{t} - x^{t-1}\right\|_2^2 + \lambda^{\mathrm{ord}}_\rho \left\|\rho^{t} - \rho^{t-1}\right\|_2^2\notag\\ &+ \lambda^{\mathrm{ord}}_\sigma(\sigma^{t} - \sigma^{t-1})^2 + \lambda_{\mathrm{obj}} \chi(x^t, x^{t-1}))
\end{align}

where $\lambda^{\mathrm{ord}}_x$, $\lambda^{\mathrm{ord}}_\rho$, $\lambda^{\mathrm{ord}}_\sigma$, $\lambda_{\mathrm{obj}}$ are positive weighting parameters. The function $\chi(x^t, x^{t-1})$ is equal to 1 if the input strokes are located on different subjects and 0 otherwise, and it is computed using the dataset segmentation masks.
Importantly, we ensure that the ordering relation between overlapping strokes is preserved, guaranteeing that both the original and reordered sequences of strokes produce the same visual output when rendered. Such problem is an instance of the Sequential Ordering Problem which we optimize following \cite{helsgaun2017lkh3}. \\

\noindent \textbf{Rendering.} To render the strokes on the canvas, we follow \cite{liu2021painttransformer} and use a \emph{parameter free} renderer. Starting from a primitive brushstroke, affine transformations are applied to obtain the foreground $I_{s^t}$ and the alpha matte $\alpha_{s^t}$ associated to $s^t\!=\!(x, \rho, \sigma, \omega)$. The canvas can be updated computing $I_c^{t}\!=\alpha_{s^t} \cdot I_{s^t} + (1 - \alpha_{s^t}) \cdot \!I_c^{t-1}$. We refer the reader to \cite{liu2021painttransformer} for additional details.

\section{Method}
\label{sec:supp_method}

\noindent \textbf{Architecture.} We report more details of the architecture, depicted in Fig. 2 of the main paper. 
Our model relies on the Transformer architecture of Vaswani \etal \cite{vaswani2017attention}, where we set the embedding dimensionality $\mathrm{d_{emb}}\!=\!256$, the number of heads in multi-head attention to 4, the dimension of the intermediate linear layer to 1024, and the dropout rate to 0.
The CNN encoder $F$ is composed of 4 convolutional blocks with residual connection and receives as input an image of size $256\times256$. The spatial resolution of the features is reduced by a factor of 2 in each block, resulting in a $16\times16$ output feature map. Following \cite{liu2021painttransformer}, we use two distinct image encoders for $I_\mathrm{ref}$ and $I_c$. The features obtained by the two input images are concatenated and projected to the embedding dimensionality $\mathrm{d_{emb}}$. %, we refer to these features as \emph{visual features}.
Similarly, the context strokes $s_c$ and the target strokes $s_t$ are projected to $\mathrm{d_{emb}}$ using a linear layer. 
The remaining components are implemented as standard transformers blocks. In particular, $C_e$ is transformer encoder with number of layers equal to 8, while $E$, $D_1$, $D_2$ are transformer decoders with number of layers equal to 6. \\

\noindent \textbf{Losses.}
We provide additional details about the computation of the losses.
%We provide additional details about the training procedure and how the losses are computed. 
The reconstruction loss component of $\mathcal{L}_{\beta\mhyphen\mathrm{VAE}}$ is computed by weighting the reconstruction error differently for each component of the stroke parameter:
%and introduce a positive constant $\lambda_{\mathrm{KL}}$ to weight the contribution of the KL divergence term \cite{higgins2017betavae}: \willi{Maybe can be moved to implementation details}
\begin{equation}
    \left\|s_t - \hat{s}_t\right\|_2^2 = \lambda_x \left\|x_t - \hat{x}_t\right\|_2^2 + \lambda_\rho \left\|\rho_t - \hat{\rho}_t\right\|_2^2 + \lambda_\sigma \left\|\sigma_t - \hat{\sigma}_t\right\|_2^2 + \lambda_\omega \left\|\omega_t - \hat{\omega}_t\right\|_2^2
\end{equation}
with $\lambda_{x}\!=\!1$, $\lambda_{\rho}\!=\!2.5\mathrm{e}{-1}$, $\lambda_{\sigma}\!=\!1$ and $\lambda_{\omega} \!=\!1$. In early experiments, we noticed that the component corresponding to the predicted color $\rho$, \emph{i.e.} $\left\|\rho_t - \hat{\rho}_t\right\|_2^2$, was difficult to jointly optimize with $\mathcal{L}_{\mathrm{col}}$, hence we reduced its weights until convergences of the two.
%When computing $\mathcal{L}_{\mathrm{col}}$, the color reconstruction loss with respect to $I_{\mathrm{ref}}$, we extract the target color $\tilde{\rho}$ from the reference image using biliner sampling, \emph{i.e.} $\tilde{\rho}\!=\!\texttt{bilinear}(I_{\mathrm{ref}},\hat{x}_t)$. Similarly, when computing $\mathcal{L}^{ref}_{\mathrm{col}}$.
The last component of our objective is the distribution matching loss $\mathcal{L}^{reg}_{\mathrm{dist}}$. We noticed that, when this loss is used, the predicted strokes may present a distorted height/width ratio. To avoid this issue, when computing this loss we exclude the size $\sigma$ and the orientation $\omega$ from the computation of features $\psi$. The same modification is applied to the SNP+ baseline for fairness of comparison.

\section{Experiments}
\label{sec:supp_experiments}

\noindent \textbf{Ablation.}  In this section, we report the ablation study conducted on \emph{ADE 20K Outdoor INP} dataset. The results are reported in Tab.~\ref{tab:ablation_ade}. Similarly to what observed on the \textit{Oxford-IIIT Pet INP} dataset in the main paper, when adding the different losses, only the full method can perform well under all the evaluation metrics, while the other configurations tend to focus either on the reference image, with low Stroke Color L2, or on the reconstructed brushstrokes, with low FSD, WD, and DTW. The ablation results on architectural components show that the full model outperforms the other configuration in terms of Stroke Color L2, FSD, FVD. Exceptions are WD and DTW, where the single-step decoder performs slightly better, and LPIPS, where the model produces more diverse predictions when the context information is removed. \\
\begin{table*}[t]
\setcounter{table}{0}
\caption{Ablation study on the \textit{ADE 20K Outdoor INP} dataset. (a) Ablation of losses. (b) Ablation of architectural choices: (i) remove context information $I_C$ and $s_c$, (ii) remove $C_e$, (iii) decode all strokes parameters with a single-step decoder}
\vspace{3mm}
\setlength{\tabcolsep}{1.0pt}
\footnotesize
    \begin{minipage}[t]{.60\textwidth}
    \captionsetup{labelformat=empty} 
    \centering
        \resizebox{0.97\linewidth}{!}{
        \begin{tabular}{lcccccccccc}
        \toprule
         & $\mathcal{L}_{\mathrm{VAE}}$ & $\mathcal{L}_{\mathrm{col}}$ & $\mathcal{L}_{\mathrm{col}}^{reg}$ & $\mathcal{L}_{\mathrm{dist}}^{reg}$ & L2$\downarrow$ & FSD$\downarrow$ & FVD$\downarrow$ & WD$\downarrow$ & DTW$\downarrow$ & LPIPS$\uparrow$\\
        \midrule
         &\cmark &\xmark & \xmark & \xmark &  0.136	& \textbf{1.64} &  11.9 & \textbf{0.032} & \textbf{0.849} & 0.038 \\
         &\cmark &\cmark & \xmark & \xmark & 0.058 & 2.44 & 7.18 & 0.034 & 0.899 & 0.031 \\
         &\cmark &\cmark & \cmark & \xmark & \textbf{0.043} & 6.84 & 8.16 & 0.040 & 0.974	& 0.028 \\
         &\cmark &\cmark & \xmark & \cmark & 0.094 & 1.92 & 10.5 & 0.033 & 0.892 & \textbf{0.044} \\
        \midrule
        Full &\cmark &\cmark&\cmark&\cmark& 0.044 & 2.04 & \textbf{6.60} & 0.034 & 0.893 & 0.033 \\
        \bottomrule
        \end{tabular}}
        \vspace{1.5mm}
        \caption{(a)}
        \label{tab:ablation_losses}
    \end{minipage}
    \begin{minipage}[t]{.40\textwidth}
    \captionsetup{labelformat=empty} 
    \centering
        \resizebox{0.99\linewidth}{!}{
        \begin{tabular}{lcccccc}
        \toprule
        Var. & L2$\downarrow$ & FSD$\downarrow$ & FVD$\downarrow$ & WD$\downarrow$ & DTW$\downarrow$ & LPIPS$\uparrow$\\
        \midrule
        (i) &  0.060 &	16.4 &	21.7 & 0.058 &	1.11 &	\textbf{0.039} \\
        (ii) &  0.050 &	2.27 &	7.45 &	0.035 &	0.907 &	0.031 \\
        (iii) &  0.052 & 2.28 & 7.12 & \textbf{0.032} & \textbf{0.868} &	0.029 \\
        %(iv) & 0.044&	2.212&	6.561&	0.034&	0.889&	0.030 \\
        \midrule
        
        Full &  \textbf{0.044} & \textbf{2.04} & \textbf{6.60} & 0.034 & 0.893 & 0.033  \\
        \bottomrule
        \vspace{-0.0mm}
        \end{tabular}}
        \vspace{1.0mm}
        \caption{(b)}
    \label{tab:ablation_architecture}
    \end{minipage}
\vspace{-2mm}
%(iv) concatenate $z$ and $c$ in the channel dimension.}
\label{tab:ablation_ade}
\end{table*}

\noindent \textbf{User study.}  We now provide details on the user study presented in the main paper. Each task of the user study consists of an HTML page divided into two sections. In the first, called the demonstration section, we show a collection of stroke sequences taken from the training set. In the second section, called the evaluation section,  we show the users two stroke sequences produced from the same reference images and stroke context, one produced with \methodname~and the other with one of the baselines. We asked the participants to select which of the two sequences of strokes presents characteristics (in terms of stoke positions, colors, and subject consistency) that are most similar to the ones of the strokes in the demonstration section.
To ease the evaluation, we produce sequences with a length of 24 strokes and render the obtained strokes in a short video.
The user study was conducted on 40 images taken from the test set of \textit{Oxford-IIIT Pet INP} dataset, from which a total of 120 tasks was generated. We collected a total of 960 votes from 8 unique users. An example of a user study task can be found at \href{run:website/user_study.html}{user\_study.html}.\\

\section{Qualitative Results}
\label{sec:supp_qualitative}
We provide additional qualitative results that complement the ones provided in the main paper. %We also provide qualitative results in the form of videos on our supplementary website (See \href{run:website/index.html}{main.html}).

In Fig. \ref{fig:ground_truth} we plot additional examples similar to the ones provided in Fig. 3 of the main paper. These qualitative results are obtained by generating, for each method, 100 predictions and showing the sequence that better matches
the ground truth in terms of L2 distance. The difference with the baselines is more evident when the painting is almost complete (e.g. first and last row). In these cases, we can notice that the baselines produce sequences that are clustered in the same location, and are not able to model the relative position between strokes as the ones provided in the dataset. Our method, instead, produces at least a prediction that is close to the ground truth sequence, showing that it is capable of better capturing the distribution of possible future strokes given the context.

In Fig. \ref{fig:diversity}, we visually assess one of the main characteristics of an INP method, \emph{i.e.} the possibility to suggest multiple continuations, from which the user can choose to continue the painting. In particular, we show different predictions of  \methodname~with a fixed context $I_c$ and $s_c$, obtained by sampling different $z_i \sim \mathcal{N}(0,1)$. In the first row of Fig. \ref{fig:diversity}, we can observe that for all the predicted continuations our model produces coherent predictions trying to add detail to the upper part of the dog, starting from the location of the last context stroke. Similarly, in the remaining examples, it can be noted how the model produces various plausible continuations focusing on the object containing the last context stroke.

Next, we compare the methods when producing longer sequences of strokes, in this specific case we set the length $k \!=\!24$. These examples, as well as additional sequences, can be visualized as videos in our supplementary website \href{run:website/sequences.html}{sequences.html}. In the first example, baseline methods tend to predict strokes that are all clustered in the same spatial location, often with high overlap. Conversely, our method can produce continuations that cover the whole cat. Note that, in this example, our method continued to paint the same object the user was painting in the context strokes and used colors consistent with the context. 
In the second example, the difference is more subtle. It is possible to notice that our method produces strokes that are more color consistent, painting first the red strokes of the house and then moving to the green ones of the grass. Vice-versa, the baselines tend to switch more times between red and green, with PT predicting blue strokes of the sky.

We produce two qualitative results to further demonstrate the capabilities of \methodname. In Fig. \ref{fig:heatmap}, we show the heatmap depicting the probability that a certain pixel will be covered by one of the next $k$ strokes predicted by the model for the current context. We estimate the probability by predicting 500 strokes continuations for the same context with the different methods. We notice that \methodname~recognizes the main objects in the reference images and tends to predict strokes on the same object as the last context strokes. This can be noted by the object outlines emerging from the heatmaps (e.g. in the first row).
From this visualization, it is possible to appreciate the diversity of the predictions that different methods can produce. Paint Transformer, being deterministic, always predicts the same strokes, while SNP and SNP+ produce strokes that are not as varied as the ones produced by \methodname.
Lastly, in \ref{fig:interpolation} we show the structure of the learned latent representation. In particular, we produce interpolation results between different sampled latent codes $z$ and provide the respective video animations in the supplementary website (See. \href{run:website/interpolations.html}{interpolations.html}). Specifically, we sample two different latent codes from the prior distribution, $z_{\mathrm{start}}, z_{\mathrm{end}} \sim \mathcal{N}(0,1)$ and we linearly interpolate between the two samples, plotting the predicted results along the interpolation path. 
It is possible to notice that the strokes smoothly transition between the two samples, changing their position but focusing on the same subject.

\begin{table*}[t]
    \centering
    
    \resizebox{0.8\linewidth}{!}{
    \setlength\tabcolsep{0pt}
    \footnotesize
    
    \begin{tabular}{ccccc}
         $I_{\text{ref}}$ & \methodname & PT & SNP & SNP+  \\

            \includegraphics[trim=2 0 0 2,clip,width=0.2\columnwidth]{supp_mat/oxford/ground_truth/Egyptian_Mau_74_reference_img.png} &
            \includegraphics[trim=2 0 0 2,clip,width=0.2\columnwidth]{supp_mat/oxford/ground_truth/Egyptian_Mau_74_our_seq_00.png} & 
            \includegraphics[trim=2 0 0 2,clip,width=0.2\columnwidth]{supp_mat/oxford/ground_truth/Egyptian_Mau_74_pt_seq.png} &
            \includegraphics[trim=2 0 0 2,clip,width=0.2\columnwidth]{supp_mat/oxford/ground_truth/Egyptian_Mau_74_snp_seq.png} &
            \includegraphics[trim=2 0 0 2,clip,width=0.2\columnwidth]{supp_mat/oxford/ground_truth/Egyptian_Mau_74_snp2_seq.png} \\
            
            \includegraphics[trim=2 0 0 2,clip,width=0.2\columnwidth]{supp_mat/oxford/ground_truth/Abyssinian_112_reference_img.png} &
            \includegraphics[trim=2 0 0 2,clip,width=0.2\columnwidth]{supp_mat/oxford/ground_truth/Abyssinian_112_our_seq_00.png} & 
            \includegraphics[trim=2 0 0 2,clip,width=0.2\columnwidth]{supp_mat/oxford/ground_truth/Abyssinian_112_pt_seq.png} &
            \includegraphics[trim=2 0 0 2,clip,width=0.2\columnwidth]{supp_mat/oxford/ground_truth/Abyssinian_112_snp_seq.png} &
            \includegraphics[trim=2 0 0 2,clip,width=0.2\columnwidth]{supp_mat/oxford/ground_truth/Abyssinian_112_snp2_seq.png} \\
            
            \includegraphics[trim=2 0 0 2,clip,width=0.2\columnwidth]{supp_mat/oxford/ground_truth/basset_hound_81_reference_img.png} &
            \includegraphics[trim=2 0 0 2,clip,width=0.2\columnwidth]{supp_mat/oxford/ground_truth/basset_hound_81_our_seq_00.png} & 
            \includegraphics[trim=2 0 0 2,clip,width=0.2\columnwidth]{supp_mat/oxford/ground_truth/basset_hound_81_pt_seq.png} &
            \includegraphics[trim=2 0 0 2,clip,width=0.2\columnwidth]{supp_mat/oxford/ground_truth/basset_hound_81_snp_seq.png} &
            \includegraphics[trim=2 0 0 2,clip,width=0.2\columnwidth]{supp_mat/oxford/ground_truth/basset_hound_81_snp2_seq.png} \\
            
            \includegraphics[trim=2 0 0 2,clip,width=0.2\columnwidth]{supp_mat/oxford/ground_truth/saint_bernard_93_reference_img.png} &
            \includegraphics[trim=2 0 0 2,clip,width=0.2\columnwidth]{supp_mat/oxford/ground_truth/saint_bernard_93_our_seq_00.png} & 
            \includegraphics[trim=2 0 0 2,clip,width=0.2\columnwidth]{supp_mat/oxford/ground_truth/saint_bernard_93_pt_seq.png} &
            \includegraphics[trim=2 0 0 2,clip,width=0.2\columnwidth]{supp_mat/oxford/ground_truth/saint_bernard_93_snp_seq.png} &
            \includegraphics[trim=2 0 0 2,clip,width=0.2\columnwidth]{supp_mat/oxford/ground_truth/saint_bernard_93_snp2_seq.png} \\
            
            \includegraphics[trim=2 0 0 2,clip,width=0.2\columnwidth]{supp_mat/ade/ground_truth/ADE_train_00002084_reference_img.png} &
            \includegraphics[trim=2 0 0 2,clip,width=0.2\columnwidth]{supp_mat/ade/ground_truth/ADE_train_00002084_our_seq_00.png} & 
            \includegraphics[trim=2 0 0 2,clip,width=0.2\columnwidth]{supp_mat/ade/ground_truth/ADE_train_00002084_pt_seq.png} &
            \includegraphics[trim=2 0 0 2,clip,width=0.2\columnwidth]{supp_mat/ade/ground_truth/ADE_train_00002084_snp_seq.png} &
            \includegraphics[trim=2 0 0 2,clip,width=0.2\columnwidth]{supp_mat/ade/ground_truth/ADE_train_00002084_snp2_seq.png} \\
            
            \includegraphics[trim=2 0 0 2,clip,width=0.2\columnwidth]{supp_mat/ade/ground_truth/ADE_train_00005219_reference_img.png} &
            \includegraphics[trim=2 0 0 2,clip,width=0.2\columnwidth]{supp_mat/ade/ground_truth/ADE_train_00005219_our_seq_00.png} & 
            \includegraphics[trim=2 0 0 2,clip,width=0.2\columnwidth]{supp_mat/ade/ground_truth/ADE_train_00005219_pt_seq.png} &
            \includegraphics[trim=2 0 0 2,clip,width=0.2\columnwidth]{supp_mat/ade/ground_truth/ADE_train_00005219_snp_seq.png} &
            \includegraphics[trim=2 0 0 2,clip,width=0.2\columnwidth]{supp_mat/ade/ground_truth/ADE_train_00005219_snp2_seq.png} \\
            
            \includegraphics[trim=2 0 0 2,clip,width=0.2\columnwidth]{supp_mat/ade/ground_truth/ADE_train_00009911_reference_img.png} &
            \includegraphics[trim=2 0 0 2,clip,width=0.2\columnwidth]{supp_mat/ade/ground_truth/ADE_train_00009911_our_seq_00.png} & 
            \includegraphics[trim=2 0 0 2,clip,width=0.2\columnwidth]{supp_mat/ade/ground_truth/ADE_train_00009911_pt_seq.png} &
            \includegraphics[trim=2 0 0 2,clip,width=0.2\columnwidth]{supp_mat/ade/ground_truth/ADE_train_00009911_snp_seq.png} &
            \includegraphics[trim=2 0 0 2,clip,width=0.2\columnwidth]{supp_mat/ade/ground_truth/ADE_train_00009911_snp2_seq.png} \\
            
            \includegraphics[trim=2 0 0 2,clip,width=0.2\columnwidth]{supp_mat/ade/ground_truth/ADE_train_00000568_reference_img.png} &
            \includegraphics[trim=2 0 0 2,clip,width=0.2\columnwidth]{supp_mat/ade/ground_truth/ADE_train_00000568_our_seq_00.png} & 
            \includegraphics[trim=2 0 0 2,clip,width=0.2\columnwidth]{supp_mat/ade/ground_truth/ADE_train_00000568_pt_seq.png} &
            \includegraphics[trim=2 0 0 2,clip,width=0.2\columnwidth]{supp_mat/ade/ground_truth/ADE_train_00000568_snp_seq.png} &
            \includegraphics[trim=2 0 0 2,clip,width=0.2\columnwidth]{supp_mat/ade/ground_truth/ADE_train_00000568_snp2_seq.png} \\

    \end{tabular}
    }
    \captionof{figure}{Qualitative comparison of \methodname~with baselines. Given the {\color{blue} context} (blue) strokes, we generate 100 {\color{red} predicted} (red) stroke sequences and plot the one that better matches the {\color{green} ground truth} (green). %Our method produces the sequence closest to the ground truth, suggesting that the distribution of predicted stroke sequences better matches the ground truth
    }
    \label{fig:ground_truth}
\end{table*}

\begin{table*}[t]
    \centering
    
    \resizebox{0.8\linewidth}{!}{
    \setlength\tabcolsep{0pt}
    \footnotesize
    
    \begin{tabular}{ccccc}
         $I_{\text{ref}}$ & $z_1$ & $z_2$ & $z_3$ & $z_4$  \\
        \includegraphics[trim=2 0 0 2,clip,width=0.2\columnwidth]{supp_mat/oxford/diversity/beagle_12_reference_img.png} & 
        \includegraphics[trim=2 0 0 2,clip,width=0.2\columnwidth]{supp_mat/oxford/diversity/beagle_12_our_seq_01.png} & 
        \includegraphics[trim=2 0 0 2,clip,width=0.2\columnwidth]{supp_mat/oxford/diversity/beagle_12_our_seq_02.png} & 
        \includegraphics[trim=2 0 0 2,clip,width=0.2\columnwidth]{supp_mat/oxford/diversity/beagle_12_our_seq_03.png} & 
        \includegraphics[trim=2 0 0 2,clip,width=0.2\columnwidth]{supp_mat/oxford/diversity/beagle_12_our_seq_04.png}  \\

        \includegraphics[trim=2 0 0 2,clip,width=0.2\columnwidth]{supp_mat/oxford/diversity/British_Shorthair_130_reference_img.png} & 
        \includegraphics[trim=2 0 0 2,clip,width=0.2\columnwidth]{supp_mat/oxford/diversity/British_Shorthair_130_our_seq_01.png} & 
        \includegraphics[trim=2 0 0 2,clip,width=0.2\columnwidth]{supp_mat/oxford/diversity/British_Shorthair_130_our_seq_02.png} & 
        \includegraphics[trim=2 0 0 2,clip,width=0.2\columnwidth]{supp_mat/oxford/diversity/British_Shorthair_130_our_seq_03.png} & 
        \includegraphics[trim=2 0 0 2,clip,width=0.2\columnwidth]{supp_mat/oxford/diversity/British_Shorthair_130_our_seq_04.png}  \\
        
        \includegraphics[trim=2 0 0 2,clip,width=0.2\columnwidth]{supp_mat/oxford/diversity/Abyssinian_206_reference_img.png} & 
        \includegraphics[trim=2 0 0 2,clip,width=0.2\columnwidth]{supp_mat/oxford/diversity/Abyssinian_206_our_seq_01.png} & 
        \includegraphics[trim=2 0 0 2,clip,width=0.2\columnwidth]{supp_mat/oxford/diversity/Abyssinian_206_our_seq_02.png} & 
        \includegraphics[trim=2 0 0 2,clip,width=0.2\columnwidth]{supp_mat/oxford/diversity/Abyssinian_206_our_seq_03.png} & 
        \includegraphics[trim=2 0 0 2,clip,width=0.2\columnwidth]{supp_mat/oxford/diversity/Abyssinian_206_our_seq_04.png}  \\
                
        \includegraphics[trim=2 0 0 2,clip,width=0.2\columnwidth]{supp_mat/oxford/diversity/german_shorthaired_153_reference_img.png} & 
        \includegraphics[trim=2 0 0 2,clip,width=0.2\columnwidth]{supp_mat/oxford/diversity/german_shorthaired_153_our_seq_01.png} & 
        \includegraphics[trim=2 0 0 2,clip,width=0.2\columnwidth]{supp_mat/oxford/diversity/german_shorthaired_153_our_seq_02.png} & 
        \includegraphics[trim=2 0 0 2,clip,width=0.2\columnwidth]{supp_mat/oxford/diversity/german_shorthaired_153_our_seq_03.png} & 
        \includegraphics[trim=2 0 0 2,clip,width=0.2\columnwidth]{supp_mat/oxford/diversity/german_shorthaired_153_our_seq_04.png}  \\
        
        \includegraphics[trim=2 0 0 2,clip,width=0.2\columnwidth]{supp_mat/ade/diversity/ADE_train_00004551_reference_img.png} & 
        \includegraphics[trim=2 0 0 2,clip,width=0.2\columnwidth]{supp_mat/ade/diversity/ADE_train_00004551_our_seq_01.png} & 
        \includegraphics[trim=2 0 0 2,clip,width=0.2\columnwidth]{supp_mat/ade/diversity/ADE_train_00004551_our_seq_02.png} &
        \includegraphics[trim=2 0 0 2,clip,width=0.2\columnwidth]{supp_mat/ade/diversity/ADE_train_00004551_our_seq_03.png} & 
        \includegraphics[trim=2 0 0 2,clip,width=0.2\columnwidth]{supp_mat/ade/diversity/ADE_train_00004551_our_seq_04.png}  \\
                 
        \includegraphics[trim=2 0 0 2,clip,width=0.2\columnwidth]{supp_mat/ade/diversity/ADE_train_00006369_reference_img.png} & 
        \includegraphics[trim=2 0 0 2,clip,width=0.2\columnwidth]{supp_mat/ade/diversity/ADE_train_00006369_our_seq_01.png} & 
        \includegraphics[trim=2 0 0 2,clip,width=0.2\columnwidth]{supp_mat/ade/diversity/ADE_train_00006369_our_seq_02.png} &
        \includegraphics[trim=2 0 0 2,clip,width=0.2\columnwidth]{supp_mat/ade/diversity/ADE_train_00006369_our_seq_03.png} & 
        \includegraphics[trim=2 0 0 2,clip,width=0.2\columnwidth]{supp_mat/ade/diversity/ADE_train_00006369_our_seq_04.png}  \\
                 
        \includegraphics[trim=2 0 0 2,clip,width=0.2\columnwidth]{supp_mat/ade/diversity/ADE_train_00007858_reference_img.png} & 
        \includegraphics[trim=2 0 0 2,clip,width=0.2\columnwidth]{supp_mat/ade/diversity/ADE_train_00007858_our_seq_01.png} & 
        \includegraphics[trim=2 0 0 2,clip,width=0.2\columnwidth]{supp_mat/ade/diversity/ADE_train_00007858_our_seq_02.png} &
        \includegraphics[trim=2 0 0 2,clip,width=0.2\columnwidth]{supp_mat/ade/diversity/ADE_train_00007858_our_seq_03.png} & 
        \includegraphics[trim=2 0 0 2,clip,width=0.2\columnwidth]{supp_mat/ade/diversity/ADE_train_00007858_our_seq_04.png}  \\
                 
        \includegraphics[trim=2 0 0 2,clip,width=0.2\columnwidth]{supp_mat/ade/diversity/ADE_train_00012101_reference_img.png} & 
        \includegraphics[trim=2 0 0 2,clip,width=0.2\columnwidth]{supp_mat/ade/diversity/ADE_train_00012101_our_seq_01.png} & 
        \includegraphics[trim=2 0 0 2,clip,width=0.2\columnwidth]{supp_mat/ade/diversity/ADE_train_00012101_our_seq_02.png} &
        \includegraphics[trim=2 0 0 2,clip,width=0.2\columnwidth]{supp_mat/ade/diversity/ADE_train_00012101_our_seq_03.png} & 
        \includegraphics[trim=2 0 0 2,clip,width=0.2\columnwidth]{supp_mat/ade/diversity/ADE_train_00012101_our_seq_04.png}  \\
         
    \end{tabular}
    }
    \vspace{2mm}
    \captionof{figure}{Diversity of proposed stroke continuations from the same context. Given a fixed {\color{blue} context} (blue), we sample different $z_i \sim \mathcal{N}(0,1)$ and plot the correspondent {\color{red} predicted} (red) strokes in different columns.} %Our method produces varied stroke suggestions that focus on the same subject as the context strokes}
    \label{fig:diversity}
\end{table*}
\begin{table*}[t]
    \centering
    
    \resizebox{\linewidth}{!}{
    \setlength\tabcolsep{0pt}
    \footnotesize
    
    \begin{tabular}{c@{\hskip 0.7mm}ccccccc}
         & $k=1$ & $k=4$ & $K=8$ & $k=12$ & $k=16$ & $k=20$ & $k=24$ \\
            % New sample
            \rotatebox{90}{\hspace{3.5mm}\methodname}  & \includegraphics[trim=2 0 0 2,clip,width=0.2\columnwidth]{supp_mat/oxford/sequence/our/0.jpg} &
            \includegraphics[trim=2 0 0 2,clip,width=0.2\columnwidth]{supp_mat/oxford/sequence/our/4.jpg} &
            \includegraphics[trim=2 0 0 2,clip,width=0.2\columnwidth]{supp_mat/oxford/sequence/our/8.jpg} &
            \includegraphics[trim=2 0 0 2,clip,width=0.2\columnwidth]{supp_mat/oxford/sequence/our/12.jpg} &
            \includegraphics[trim=2 0 0 2,clip,width=0.2\columnwidth]{supp_mat/oxford/sequence/our/16.jpg} &
            \includegraphics[trim=2 0 0 2,clip,width=0.2\columnwidth]{supp_mat/oxford/sequence/our/20.jpg} &
            \includegraphics[trim=2 0 0 2,clip,width=0.2\columnwidth]{supp_mat/oxford/sequence/our/23.jpg} \\
                     
            \rotatebox{90}{\hspace{3.5mm}PT} &\includegraphics[trim=2 0 0 2,clip,width=0.2\columnwidth]{supp_mat/oxford/sequence/pt/0.jpg} &
            \includegraphics[trim=2 0 0 2,clip,width=0.2\columnwidth]{supp_mat/oxford/sequence/pt/4.jpg} &
            \includegraphics[trim=2 0 0 2,clip,width=0.2\columnwidth]{supp_mat/oxford/sequence/pt/8.jpg} &
            \includegraphics[trim=2 0 0 2,clip,width=0.2\columnwidth]{supp_mat/oxford/sequence/pt/12.jpg} &
            \includegraphics[trim=2 0 0 2,clip,width=0.2\columnwidth]{supp_mat/oxford/sequence/pt/16.jpg} &
            \includegraphics[trim=2 0 0 2,clip,width=0.2\columnwidth]{supp_mat/oxford/sequence/pt/20.jpg} &
            \includegraphics[trim=2 0 0 2,clip,width=0.2\columnwidth]{supp_mat/oxford/sequence/pt/23.jpg} \\

            \rotatebox{90}{\hspace{3.5mm}SNP} &\includegraphics[trim=2 0 0 2,clip,width=0.2\columnwidth]{supp_mat/oxford/sequence/snp/0.jpg} &
            \includegraphics[trim=2 0 0 2,clip,width=0.2\columnwidth]{supp_mat/oxford/sequence/snp/4.jpg} &
            \includegraphics[trim=2 0 0 2,clip,width=0.2\columnwidth]{supp_mat/oxford/sequence/snp/8.jpg} &
            \includegraphics[trim=2 0 0 2,clip,width=0.2\columnwidth]{supp_mat/oxford/sequence/snp/12.jpg} &
            \includegraphics[trim=2 0 0 2,clip,width=0.2\columnwidth]{supp_mat/oxford/sequence/snp/16.jpg} &
            \includegraphics[trim=2 0 0 2,clip,width=0.2\columnwidth]{supp_mat/oxford/sequence/snp/20.jpg} &
            \includegraphics[trim=2 0 0 2,clip,width=0.2\columnwidth]{supp_mat/oxford/sequence/snp/23.jpg} \\
            
            \rotatebox{90}{\hspace{3.5mm}SNP+} &\includegraphics[trim=2 0 0 2,clip,width=0.2\columnwidth]{supp_mat/oxford/sequence/snp2/0.jpg} &
            \includegraphics[trim=2 0 0 2,clip,width=0.2\columnwidth]{supp_mat/oxford/sequence/snp2/4.jpg} &
            \includegraphics[trim=2 0 0 2,clip,width=0.2\columnwidth]{supp_mat/oxford/sequence/snp2/8.jpg} &
            \includegraphics[trim=2 0 0 2,clip,width=0.2\columnwidth]{supp_mat/oxford/sequence/snp2/12.jpg} &
            \includegraphics[trim=2 0 0 2,clip,width=0.2\columnwidth]{supp_mat/oxford/sequence/snp2/16.jpg} &
            \includegraphics[trim=2 0 0 2,clip,width=0.2\columnwidth]{supp_mat/oxford/sequence/snp2/20.jpg} &
            \includegraphics[trim=2 0 0 2,clip,width=0.2\columnwidth]{supp_mat/oxford/sequence/snp2/23.jpg} \\
            
            \rotatebox{90}{\hspace{3.5mm}\methodname} &\includegraphics[trim=2 0 0 2,clip,width=0.2\columnwidth]{supp_mat/ade/sequence/our/0.jpg} &
            \includegraphics[trim=2 0 0 2,clip,width=0.2\columnwidth]{supp_mat/ade/sequence/our/4.jpg} &
            \includegraphics[trim=2 0 0 2,clip,width=0.2\columnwidth]{supp_mat/ade/sequence/our/8.jpg} &
            \includegraphics[trim=2 0 0 2,clip,width=0.2\columnwidth]{supp_mat/ade/sequence/our/12.jpg} &
            \includegraphics[trim=2 0 0 2,clip,width=0.2\columnwidth]{supp_mat/ade/sequence/our/16.jpg} &
            \includegraphics[trim=2 0 0 2,clip,width=0.2\columnwidth]{supp_mat/ade/sequence/our/20.jpg} &
            \includegraphics[trim=2 0 0 2,clip,width=0.2\columnwidth]{supp_mat/ade/sequence/our/23.jpg} \\

            \rotatebox{90}{\hspace{4mm}PT} & \includegraphics[trim=2 0 0 2,clip,width=0.2\columnwidth]{supp_mat/ade/sequence/pt/0.jpg} &
            \includegraphics[trim=2 0 0 2,clip,width=0.2\columnwidth]{supp_mat/ade/sequence/pt/4.jpg} &
            \includegraphics[trim=2 0 0 2,clip,width=0.2\columnwidth]{supp_mat/ade/sequence/pt/8.jpg} &
            \includegraphics[trim=2 0 0 2,clip,width=0.2\columnwidth]{supp_mat/ade/sequence/pt/12.jpg} &
            \includegraphics[trim=2 0 0 2,clip,width=0.2\columnwidth]{supp_mat/ade/sequence/pt/16.jpg} &
            \includegraphics[trim=2 0 0 2,clip,width=0.2\columnwidth]{supp_mat/ade/sequence/pt/20.jpg} &
            \includegraphics[trim=2 0 0 2,clip,width=0.2\columnwidth]{supp_mat/ade/sequence/pt/23.jpg} \\

            \rotatebox{90}{\hspace{3.5mm}SNP} &\includegraphics[trim=2 0 0 2,clip,width=0.2\columnwidth]{supp_mat/ade/sequence/snp/0.jpg} &
            \includegraphics[trim=2 0 0 2,clip,width=0.2\columnwidth]{supp_mat/ade/sequence/snp/4.jpg} &
            \includegraphics[trim=2 0 0 2,clip,width=0.2\columnwidth]{supp_mat/ade/sequence/snp/8.jpg} &
            \includegraphics[trim=2 0 0 2,clip,width=0.2\columnwidth]{supp_mat/ade/sequence/snp/12.jpg} &
            \includegraphics[trim=2 0 0 2,clip,width=0.2\columnwidth]{supp_mat/ade/sequence/snp/16.jpg} &
            \includegraphics[trim=2 0 0 2,clip,width=0.2\columnwidth]{supp_mat/ade/sequence/snp/20.jpg} &
            \includegraphics[trim=2 0 0 2,clip,width=0.2\columnwidth]{supp_mat/ade/sequence/snp/23.jpg} \\
            
            \rotatebox{90}{\hspace{3.5mm}SNP+} & \includegraphics[trim=2 0 0 2,clip,width=0.2\columnwidth]{supp_mat/ade/sequence/snp2/0.jpg} &
            \includegraphics[trim=2 0 0 2,clip,width=0.2\columnwidth]{supp_mat/ade/sequence/snp2/4.jpg} &
            \includegraphics[trim=2 0 0 2,clip,width=0.2\columnwidth]{supp_mat/ade/sequence/snp2/8.jpg} &
            \includegraphics[trim=2 0 0 2,clip,width=0.2\columnwidth]{supp_mat/ade/sequence/snp2/12.jpg} &
            \includegraphics[trim=2 0 0 2,clip,width=0.2\columnwidth]{supp_mat/ade/sequence/snp2/16.jpg} &
            \includegraphics[trim=2 0 0 2,clip,width=0.2\columnwidth]{supp_mat/ade/sequence/snp2/20.jpg} &
            \includegraphics[trim=2 0 0 2,clip,width=0.2\columnwidth]{supp_mat/ade/sequence/snp2/23.jpg} \\
        
    \end{tabular}
    }
    \vspace{2mm}
    \captionof{figure}{Visualization of prediction results for a sequence of 24 predicted strokes.}
    \label{fig:sequence}
\end{table*}

\begin{table*}[t]
    \centering
    
    \resizebox{\linewidth}{!}{
    \setlength\tabcolsep{0pt}
    \footnotesize
    
    \begin{tabular}{ccccccc}
         $I_{\text{ref}}$ & $\alpha\!=\!0$ & $\alpha\!=\!0.2$ & $\alpha\!=\!0.4$ & $\alpha\!=\!0.6$ & $\alpha\!=\!0.8$ & $\alpha\!=\!1$ \\
        \includegraphics[trim=2 0 0 2,clip,width=0.2\columnwidth]{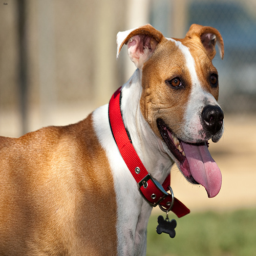} &
       \includegraphics[trim=2 0 0 2,clip,width=0.2\columnwidth]{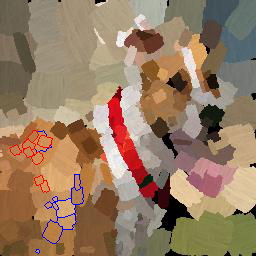} &
       \includegraphics[trim=2 0 0 2,clip,width=0.2\columnwidth]{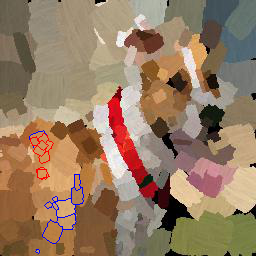} &
       \includegraphics[trim=2 0 0 2,clip,width=0.2\columnwidth]{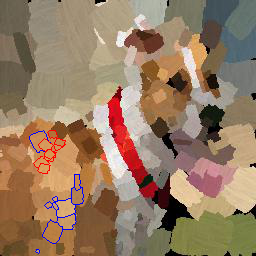} &
       \includegraphics[trim=2 0 0 2,clip,width=0.2\columnwidth]{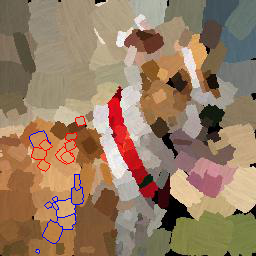} &
       \includegraphics[trim=2 0 0 2,clip,width=0.2\columnwidth]{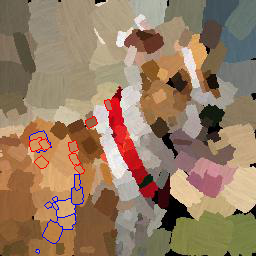} &
       \includegraphics[trim=2 0 0 2,clip,width=0.2\columnwidth]{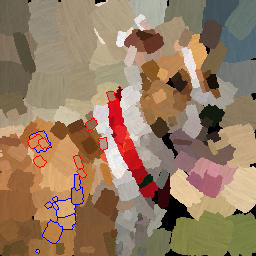} \\
       
        \includegraphics[trim=2 0 0 2,clip,width=0.2\columnwidth]{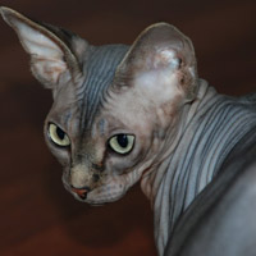} &
       \includegraphics[trim=2 0 0 2,clip,width=0.2\columnwidth]{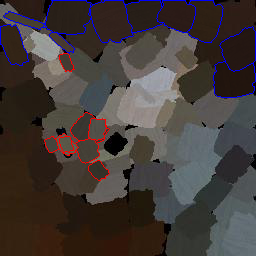} &
       \includegraphics[trim=2 0 0 2,clip,width=0.2\columnwidth]{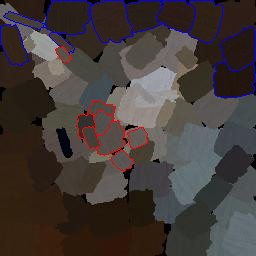} &
       \includegraphics[trim=2 0 0 2,clip,width=0.2\columnwidth]{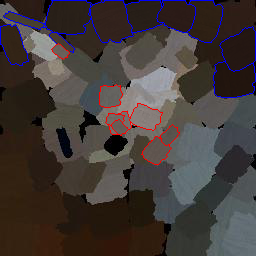} &
       \includegraphics[trim=2 0 0 2,clip,width=0.2\columnwidth]{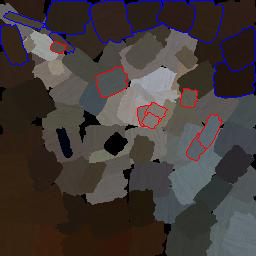} &
       \includegraphics[trim=2 0 0 2,clip,width=0.2\columnwidth]{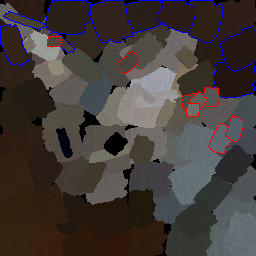} &
       \includegraphics[trim=2 0 0 2,clip,width=0.2\columnwidth]{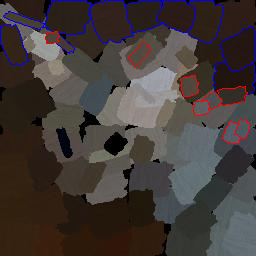} \\
       
       \includegraphics[trim=2 0 0 2,clip,width=0.2\columnwidth]{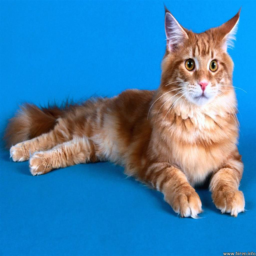} &
       \includegraphics[trim=2 0 0 2,clip,width=0.2\columnwidth]{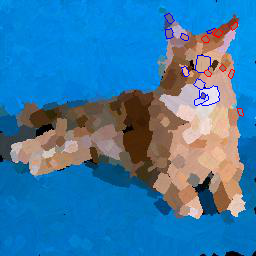} &
       \includegraphics[trim=2 0 0 2,clip,width=0.2\columnwidth]{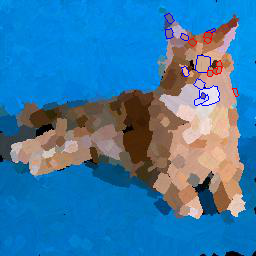} &
       \includegraphics[trim=2 0 0 2,clip,width=0.2\columnwidth]{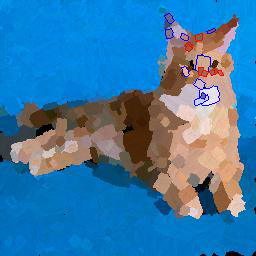} &
       \includegraphics[trim=2 0 0 2,clip,width=0.2\columnwidth]{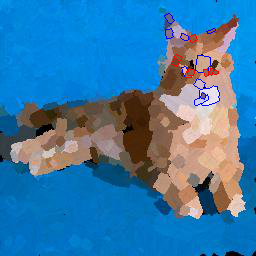} &
       \includegraphics[trim=2 0 0 2,clip,width=0.2\columnwidth]{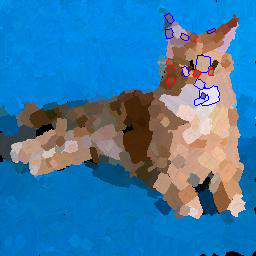} &
       \includegraphics[trim=2 0 0 2,clip,width=0.2\columnwidth]{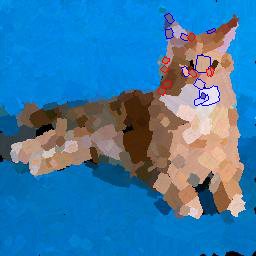} \\
       
       \includegraphics[trim=2 0 0 2,clip,width=0.2\columnwidth]{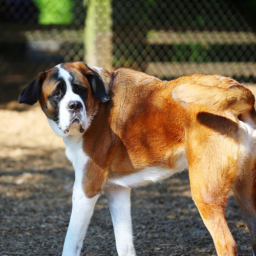} &
       \includegraphics[trim=2 0 0 2,clip,width=0.2\columnwidth]{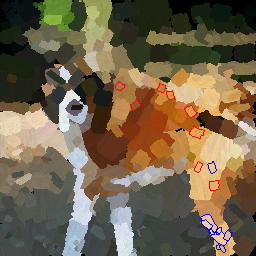} &
       \includegraphics[trim=2 0 0 2,clip,width=0.2\columnwidth]{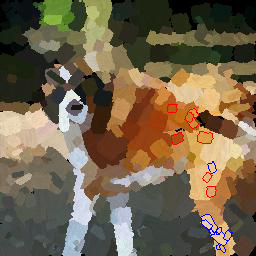} &
       \includegraphics[trim=2 0 0 2,clip,width=0.2\columnwidth]{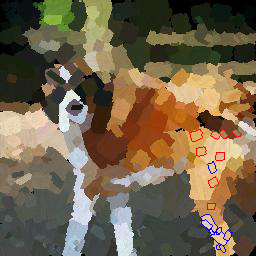} &
       \includegraphics[trim=2 0 0 2,clip,width=0.2\columnwidth]{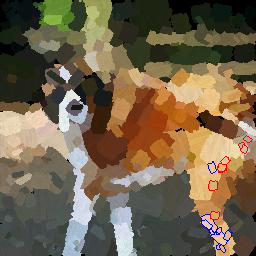} &
       \includegraphics[trim=2 0 0 2,clip,width=0.2\columnwidth]{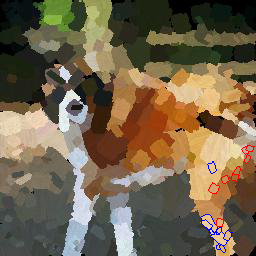} &
       \includegraphics[trim=2 0 0 2,clip,width=0.2\columnwidth]{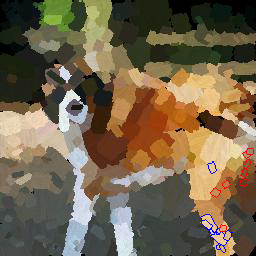} \\

        \includegraphics[trim=2 0 0 2,clip,width=0.2\columnwidth]{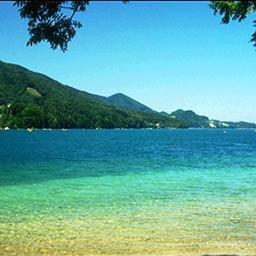} &
        \includegraphics[trim=2 0 0 2,clip,width=0.2\columnwidth]{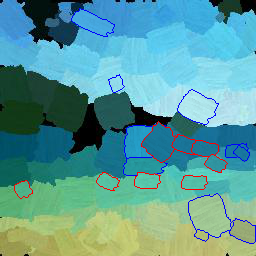} &
        \includegraphics[trim=2 0 0 2,clip,width=0.2\columnwidth]{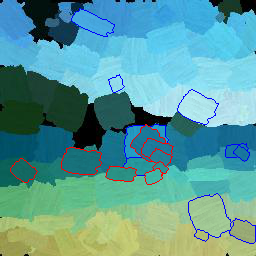} &
        \includegraphics[trim=2 0 0 2,clip,width=0.2\columnwidth]{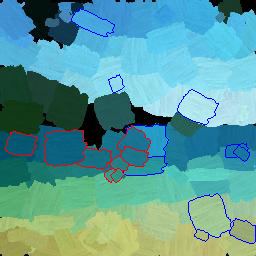} &
        \includegraphics[trim=2 0 0 2,clip,width=0.2\columnwidth]{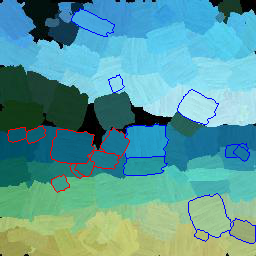} &
        \includegraphics[trim=2 0 0 2,clip,width=0.2\columnwidth]{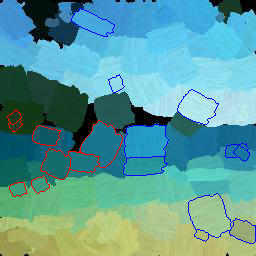} &
        \includegraphics[trim=2 0 0 2,clip,width=0.2\columnwidth]{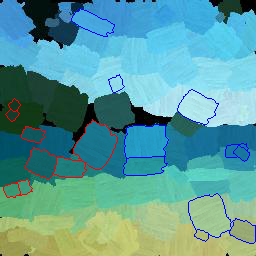} \\
        
        \includegraphics[trim=2 0 0 2,clip,width=0.2\columnwidth]{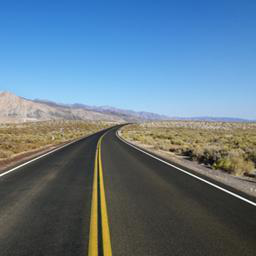} &
        \includegraphics[trim=2 0 0 2,clip,width=0.2\columnwidth]{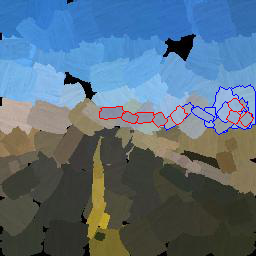} &
        \includegraphics[trim=2 0 0 2,clip,width=0.2\columnwidth]{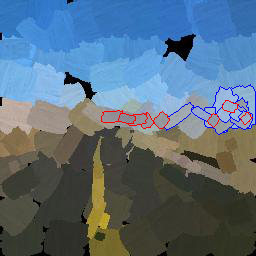} &
        \includegraphics[trim=2 0 0 2,clip,width=0.2\columnwidth]{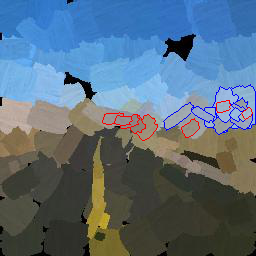} &
        \includegraphics[trim=2 0 0 2,clip,width=0.2\columnwidth]{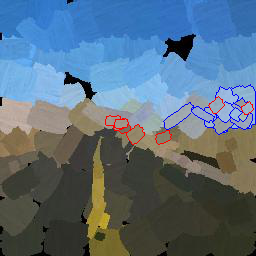} &
        \includegraphics[trim=2 0 0 2,clip,width=0.2\columnwidth]{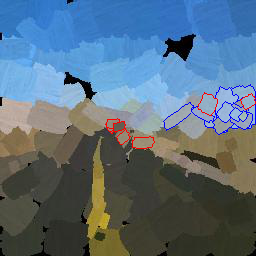} &
        \includegraphics[trim=2 0 0 2,clip,width=0.2\columnwidth]{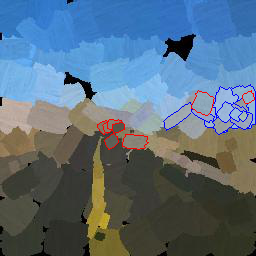} \\
        
        \includegraphics[trim=2 0 0 2,clip,width=0.2\columnwidth]{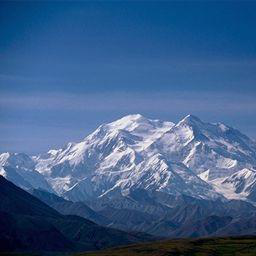} &
        \includegraphics[trim=2 0 0 2,clip,width=0.2\columnwidth]{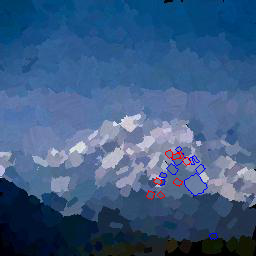} &
        \includegraphics[trim=2 0 0 2,clip,width=0.2\columnwidth]{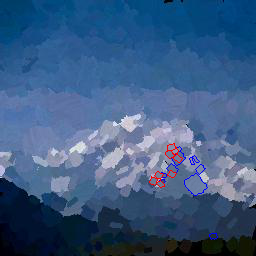} &
        \includegraphics[trim=2 0 0 2,clip,width=0.2\columnwidth]{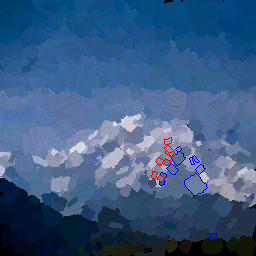} &
        \includegraphics[trim=2 0 0 2,clip,width=0.2\columnwidth]{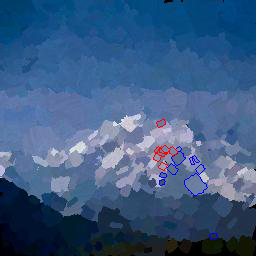} &
        \includegraphics[trim=2 0 0 2,clip,width=0.2\columnwidth]{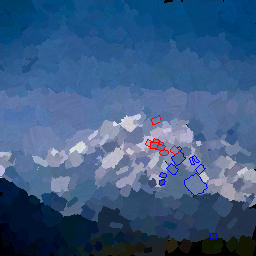} &
        \includegraphics[trim=2 0 0 2,clip,width=0.2\columnwidth]{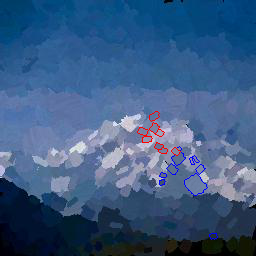} \\
        
        \includegraphics[trim=2 0 0 2,clip,width=0.2\columnwidth]{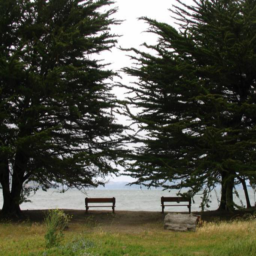} &
        \includegraphics[trim=2 0 0 2,clip,width=0.2\columnwidth]{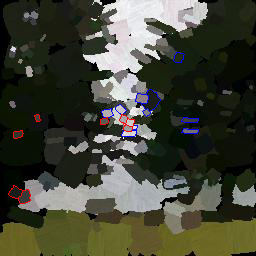} &
        \includegraphics[trim=2 0 0 2,clip,width=0.2\columnwidth]{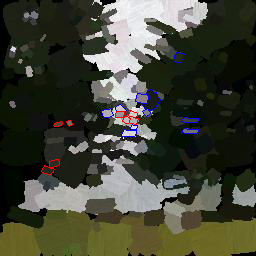} &
        \includegraphics[trim=2 0 0 2,clip,width=0.2\columnwidth]{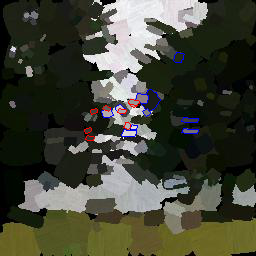} &
        \includegraphics[trim=2 0 0 2,clip,width=0.2\columnwidth]{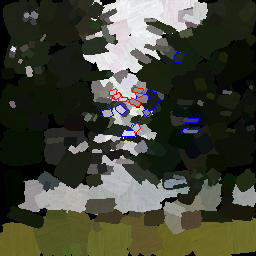} &
        \includegraphics[trim=2 0 0 2,clip,width=0.2\columnwidth]{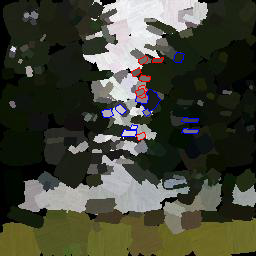} &
        \includegraphics[trim=2 0 0 2,clip,width=0.2\columnwidth]{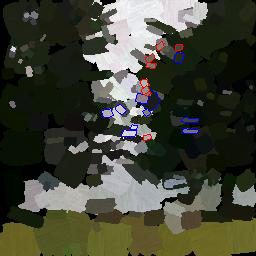} \\
    \end{tabular}
    }
    \vspace{2mm}
    \captionof{figure}{Latent code $z$ interpolation results. For each image, we sample two latent codes  $z_{\mathrm{start}}, z_{\mathrm{end}} \sim \mathcal{N}(0,1)$ and linearly interpolate, obtaining $z_i = (1 - \alpha) \cdot z_{\mathrm{start}} + \alpha \cdot z_{\mathrm{end}}$. The strokes smoothly transition changing position but focusing on the same object.}
    \label{fig:interpolation}
\end{table*}
\begin{table*}[t]
    \centering
    
    \resizebox{0.9\linewidth}{!}{
    \setlength\tabcolsep{0pt}
    \footnotesize
    
    \begin{tabular}{ccccc}
         $I_{\text{c}}$ & \methodname & PT & SNP & SNP+  \\

            \includegraphics[trim=2 0 0 2,clip,width=0.2\columnwidth]{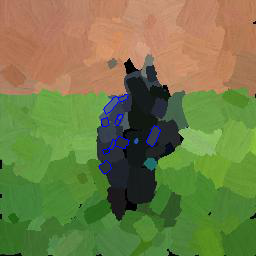} &
            \includegraphics[trim=2 0 0 2,clip,width=0.2\columnwidth]{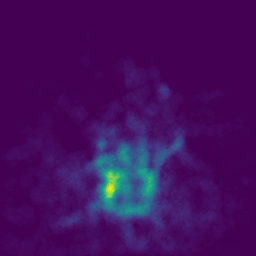} &
            \includegraphics[trim=2 0 0 2,clip,width=0.2\columnwidth]{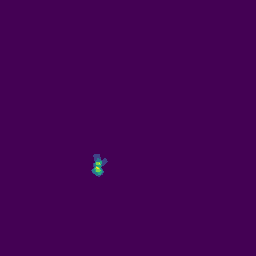} &
            \includegraphics[trim=2 0 0 2,clip,width=0.2\columnwidth]{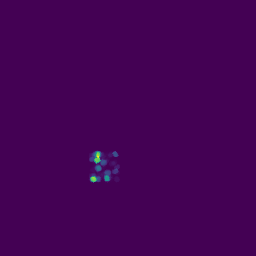} &
            \includegraphics[trim=2 0 0 2,clip,width=0.2\columnwidth]{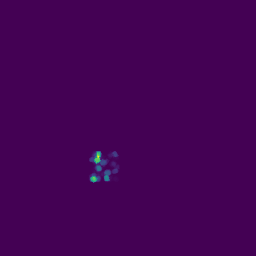} \\
            
            \includegraphics[trim=2 0 0 2,clip,width=0.2\columnwidth]{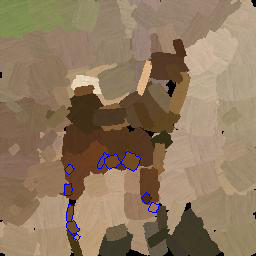} &
            \includegraphics[trim=2 0 0 2,clip,width=0.2\columnwidth]{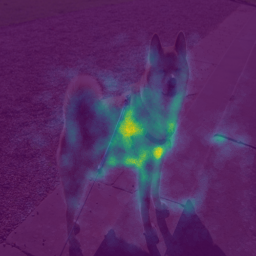} &
            \includegraphics[trim=2 0 0 2,clip,width=0.2\columnwidth]{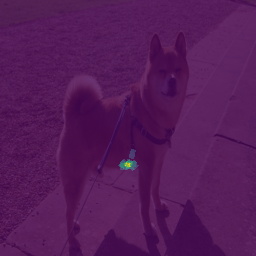} &
            \includegraphics[trim=2 0 0 2,clip,width=0.2\columnwidth]{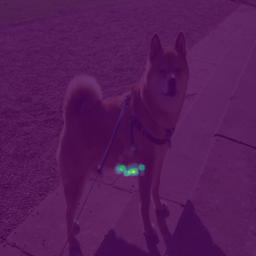} &
            \includegraphics[trim=2 0 0 2,clip,width=0.2\columnwidth]{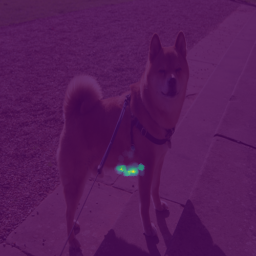} \\
            
            \includegraphics[trim=2 0 0 2,clip,width=0.2\columnwidth]{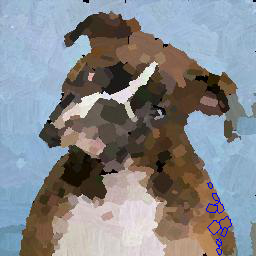} &
            \includegraphics[trim=2 0 0 2,clip,width=0.2\columnwidth]{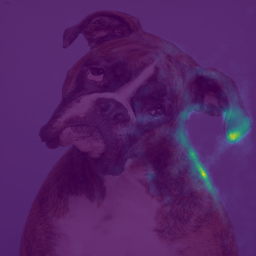} &
            \includegraphics[trim=2 0 0 2,clip,width=0.2\columnwidth]{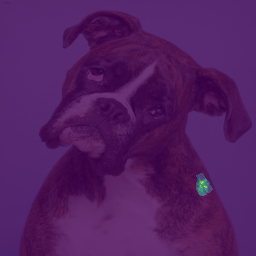} &
            \includegraphics[trim=2 0 0 2,clip,width=0.2\columnwidth]{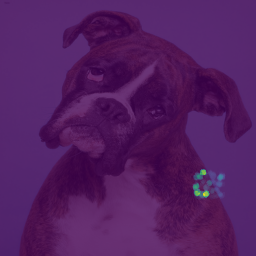} &
            \includegraphics[trim=2 0 0 2,clip,width=0.2\columnwidth]{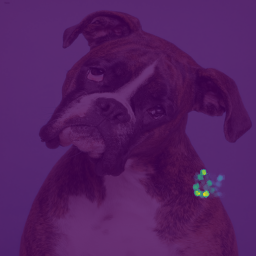} \\
         
            \includegraphics[trim=2 0 0 2,clip,width=0.2\columnwidth]{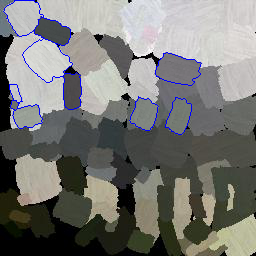} &
            \includegraphics[trim=2 0 0 2,clip,width=0.2\columnwidth]{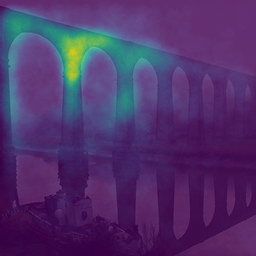} &
            \includegraphics[trim=2 0 0 2,clip,width=0.2\columnwidth]{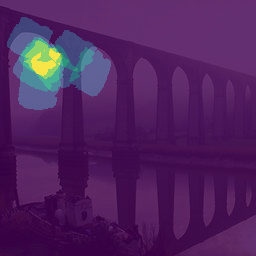} &
            \includegraphics[trim=2 0 0 2,clip,width=0.2\columnwidth]{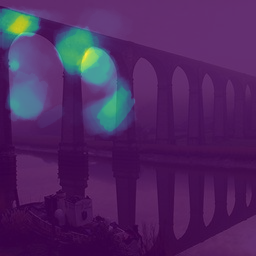} &
            \includegraphics[trim=2 0 0 2,clip,width=0.2\columnwidth]{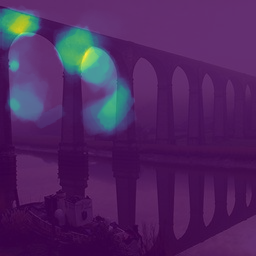}  \\
            
            \includegraphics[trim=2 0 0 2,clip,width=0.2\columnwidth]{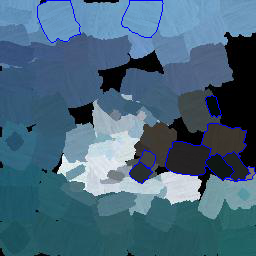} &
            \includegraphics[trim=2 0 0 2,clip,width=0.2\columnwidth]{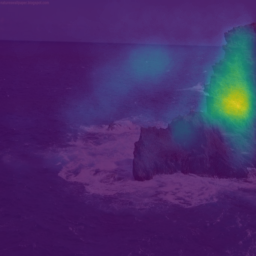} &
            \includegraphics[trim=2 0 0 2,clip,width=0.2\columnwidth]{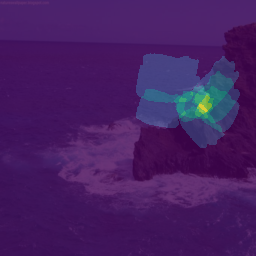} &
            \includegraphics[trim=2 0 0 2,clip,width=0.2\columnwidth]{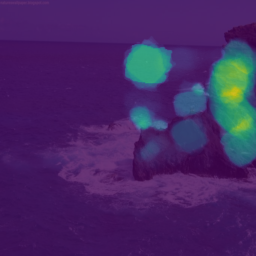} &
            \includegraphics[trim=2 0 0 2,clip,width=0.2\columnwidth]{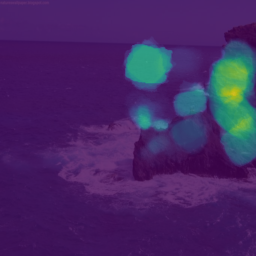}  \\
            
            \includegraphics[trim=2 0 0 2,clip,width=0.2\columnwidth]{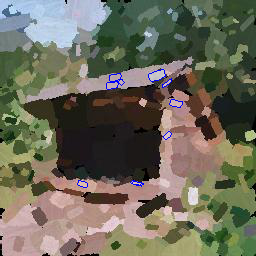} &
            \includegraphics[trim=2 0 0 2,clip,width=0.2\columnwidth]{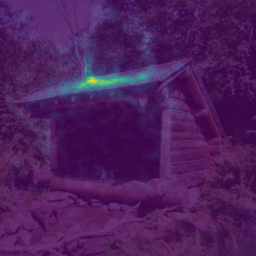} &
            \includegraphics[trim=2 0 0 2,clip,width=0.2\columnwidth]{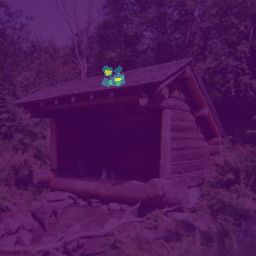} &
            \includegraphics[trim=2 0 0 2,clip,width=0.2\columnwidth]{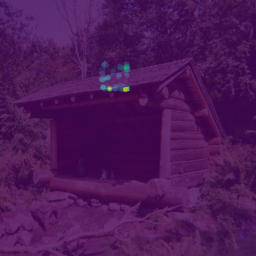} &
            \includegraphics[trim=2 0 0 2,clip,width=0.2\columnwidth]{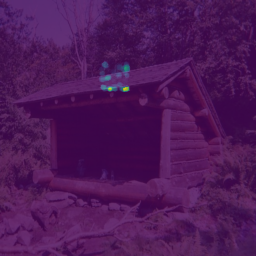}  \\

    \end{tabular}
    }
    \vspace{2mm}
    \captionof{figure}{Next predicted stroke probability distribution. For each method, we show the probability that a given pixel will be occupied by a predicted stroke for the given context. \methodname~predicts strokes that tend to focus on the same object as the context stroke and its outline emerges from the probability distribution.}
    \label{fig:heatmap}
    \vspace{-7mm}
\end{table*}
