# Supplementary material for: Interactive Neural Painting
Source: arXiv:2307.16441 source file (2023-07-31)
Supplement: Supplementary file 3 [file diversity.tex]

\begin{table*}[t]
    \centering
    
    \resizebox{0.8\linewidth}{!}{
    \setlength\tabcolsep{0pt}
    \footnotesize
    
    \begin{tabular}{ccccc}
         $I_{\text{ref}}$ & $z_1$ & $z_2$ & $z_3$ & $z_4$  \\
        \includegraphics[trim=2 0 0 2,clip,width=0.2\columnwidth]{supp_mat/oxford/diversity/beagle_12_reference_img.png} & 
        \includegraphics[trim=2 0 0 2,clip,width=0.2\columnwidth]{supp_mat/oxford/diversity/beagle_12_our_seq_01.png} & 
        \includegraphics[trim=2 0 0 2,clip,width=0.2\columnwidth]{supp_mat/oxford/diversity/beagle_12_our_seq_02.png} & 
        \includegraphics[trim=2 0 0 2,clip,width=0.2\columnwidth]{supp_mat/oxford/diversity/beagle_12_our_seq_03.png} & 
        \includegraphics[trim=2 0 0 2,clip,width=0.2\columnwidth]{supp_mat/oxford/diversity/beagle_12_our_seq_04.png}  \\

        \includegraphics[trim=2 0 0 2,clip,width=0.2\columnwidth]{supp_mat/oxford/diversity/British_Shorthair_130_reference_img.png} & 
        \includegraphics[trim=2 0 0 2,clip,width=0.2\columnwidth]{supp_mat/oxford/diversity/British_Shorthair_130_our_seq_01.png} & 
        \includegraphics[trim=2 0 0 2,clip,width=0.2\columnwidth]{supp_mat/oxford/diversity/British_Shorthair_130_our_seq_02.png} & 
        \includegraphics[trim=2 0 0 2,clip,width=0.2\columnwidth]{supp_mat/oxford/diversity/British_Shorthair_130_our_seq_03.png} & 
        \includegraphics[trim=2 0 0 2,clip,width=0.2\columnwidth]{supp_mat/oxford/diversity/British_Shorthair_130_our_seq_04.png}  \\
        
        \includegraphics[trim=2 0 0 2,clip,width=0.2\columnwidth]{supp_mat/oxford/diversity/Abyssinian_206_reference_img.png} & 
        \includegraphics[trim=2 0 0 2,clip,width=0.2\columnwidth]{supp_mat/oxford/diversity/Abyssinian_206_our_seq_01.png} & 
        \includegraphics[trim=2 0 0 2,clip,width=0.2\columnwidth]{supp_mat/oxford/diversity/Abyssinian_206_our_seq_02.png} & 
        \includegraphics[trim=2 0 0 2,clip,width=0.2\columnwidth]{supp_mat/oxford/diversity/Abyssinian_206_our_seq_03.png} & 
        \includegraphics[trim=2 0 0 2,clip,width=0.2\columnwidth]{supp_mat/oxford/diversity/Abyssinian_206_our_seq_04.png}  \\
                
        \includegraphics[trim=2 0 0 2,clip,width=0.2\columnwidth]{supp_mat/oxford/diversity/german_shorthaired_153_reference_img.png} & 
        \includegraphics[trim=2 0 0 2,clip,width=0.2\columnwidth]{supp_mat/oxford/diversity/german_shorthaired_153_our_seq_01.png} & 
        \includegraphics[trim=2 0 0 2,clip,width=0.2\columnwidth]{supp_mat/oxford/diversity/german_shorthaired_153_our_seq_02.png} & 
        \includegraphics[trim=2 0 0 2,clip,width=0.2\columnwidth]{supp_mat/oxford/diversity/german_shorthaired_153_our_seq_03.png} & 
        \includegraphics[trim=2 0 0 2,clip,width=0.2\columnwidth]{supp_mat/oxford/diversity/german_shorthaired_153_our_seq_04.png}  \\
        
        \includegraphics[trim=2 0 0 2,clip,width=0.2\columnwidth]{supp_mat/ade/diversity/ADE_train_00004551_reference_img.png} & 
        \includegraphics[trim=2 0 0 2,clip,width=0.2\columnwidth]{supp_mat/ade/diversity/ADE_train_00004551_our_seq_01.png} & 
        \includegraphics[trim=2 0 0 2,clip,width=0.2\columnwidth]{supp_mat/ade/diversity/ADE_train_00004551_our_seq_02.png} &
        \includegraphics[trim=2 0 0 2,clip,width=0.2\columnwidth]{supp_mat/ade/diversity/ADE_train_00004551_our_seq_03.png} & 
        \includegraphics[trim=2 0 0 2,clip,width=0.2\columnwidth]{supp_mat/ade/diversity/ADE_train_00004551_our_seq_04.png}  \\
                 
        \includegraphics[trim=2 0 0 2,clip,width=0.2\columnwidth]{supp_mat/ade/diversity/ADE_train_00006369_reference_img.png} & 
        \includegraphics[trim=2 0 0 2,clip,width=0.2\columnwidth]{supp_mat/ade/diversity/ADE_train_00006369_our_seq_01.png} & 
        \includegraphics[trim=2 0 0 2,clip,width=0.2\columnwidth]{supp_mat/ade/diversity/ADE_train_00006369_our_seq_02.png} &
        \includegraphics[trim=2 0 0 2,clip,width=0.2\columnwidth]{supp_mat/ade/diversity/ADE_train_00006369_our_seq_03.png} & 
        \includegraphics[trim=2 0 0 2,clip,width=0.2\columnwidth]{supp_mat/ade/diversity/ADE_train_00006369_our_seq_04.png}  \\
                 
        \includegraphics[trim=2 0 0 2,clip,width=0.2\columnwidth]{supp_mat/ade/diversity/ADE_train_00007858_reference_img.png} & 
        \includegraphics[trim=2 0 0 2,clip,width=0.2\columnwidth]{supp_mat/ade/diversity/ADE_train_00007858_our_seq_01.png} & 
        \includegraphics[trim=2 0 0 2,clip,width=0.2\columnwidth]{supp_mat/ade/diversity/ADE_train_00007858_our_seq_02.png} &
        \includegraphics[trim=2 0 0 2,clip,width=0.2\columnwidth]{supp_mat/ade/diversity/ADE_train_00007858_our_seq_03.png} & 
        \includegraphics[trim=2 0 0 2,clip,width=0.2\columnwidth]{supp_mat/ade/diversity/ADE_train_00007858_our_seq_04.png}  \\
                 
        \includegraphics[trim=2 0 0 2,clip,width=0.2\columnwidth]{supp_mat/ade/diversity/ADE_train_00012101_reference_img.png} & 
        \includegraphics[trim=2 0 0 2,clip,width=0.2\columnwidth]{supp_mat/ade/diversity/ADE_train_00012101_our_seq_01.png} & 
        \includegraphics[trim=2 0 0 2,clip,width=0.2\columnwidth]{supp_mat/ade/diversity/ADE_train_00012101_our_seq_02.png} &
        \includegraphics[trim=2 0 0 2,clip,width=0.2\columnwidth]{supp_mat/ade/diversity/ADE_train_00012101_our_seq_03.png} & 
        \includegraphics[trim=2 0 0 2,clip,width=0.2\columnwidth]{supp_mat/ade/diversity/ADE_train_00012101_our_seq_04.png}  \\
         
    \end{tabular}
    }
    \vspace{2mm}
    \captionof{figure}{Diversity of proposed stroke continuations from the same context. Given a fixed {\color{blue} context} (blue), we sample different $z_i \sim \mathcal{N}(0,1)$ and plot the correspondent {\color{red} predicted} (red) strokes in different columns.} %Our method produces varied stroke suggestions that focus on the same subject as the context strokes}
    \label{fig:diversity}
\end{table*}
