# Supplementary material for: Interactive Neural Painting
Source: arXiv:2307.16441 source file (2023-07-31)
Supplement: Supplementary file 4 [file ground_truth.tex]

\begin{table*}[t]
    \centering
    
    \resizebox{0.8\linewidth}{!}{
    \setlength\tabcolsep{0pt}
    \footnotesize
    
    \begin{tabular}{ccccc}
         $I_{\text{ref}}$ & \methodname & PT & SNP & SNP+  \\

            \includegraphics[trim=2 0 0 2,clip,width=0.2\columnwidth]{supp_mat/oxford/ground_truth/Egyptian_Mau_74_reference_img.png} &
            \includegraphics[trim=2 0 0 2,clip,width=0.2\columnwidth]{supp_mat/oxford/ground_truth/Egyptian_Mau_74_our_seq_00.png} & 
            \includegraphics[trim=2 0 0 2,clip,width=0.2\columnwidth]{supp_mat/oxford/ground_truth/Egyptian_Mau_74_pt_seq.png} &
            \includegraphics[trim=2 0 0 2,clip,width=0.2\columnwidth]{supp_mat/oxford/ground_truth/Egyptian_Mau_74_snp_seq.png} &
            \includegraphics[trim=2 0 0 2,clip,width=0.2\columnwidth]{supp_mat/oxford/ground_truth/Egyptian_Mau_74_snp2_seq.png} \\
            
            \includegraphics[trim=2 0 0 2,clip,width=0.2\columnwidth]{supp_mat/oxford/ground_truth/Abyssinian_112_reference_img.png} &
            \includegraphics[trim=2 0 0 2,clip,width=0.2\columnwidth]{supp_mat/oxford/ground_truth/Abyssinian_112_our_seq_00.png} & 
            \includegraphics[trim=2 0 0 2,clip,width=0.2\columnwidth]{supp_mat/oxford/ground_truth/Abyssinian_112_pt_seq.png} &
            \includegraphics[trim=2 0 0 2,clip,width=0.2\columnwidth]{supp_mat/oxford/ground_truth/Abyssinian_112_snp_seq.png} &
            \includegraphics[trim=2 0 0 2,clip,width=0.2\columnwidth]{supp_mat/oxford/ground_truth/Abyssinian_112_snp2_seq.png} \\
            
            \includegraphics[trim=2 0 0 2,clip,width=0.2\columnwidth]{supp_mat/oxford/ground_truth/basset_hound_81_reference_img.png} &
            \includegraphics[trim=2 0 0 2,clip,width=0.2\columnwidth]{supp_mat/oxford/ground_truth/basset_hound_81_our_seq_00.png} & 
            \includegraphics[trim=2 0 0 2,clip,width=0.2\columnwidth]{supp_mat/oxford/ground_truth/basset_hound_81_pt_seq.png} &
            \includegraphics[trim=2 0 0 2,clip,width=0.2\columnwidth]{supp_mat/oxford/ground_truth/basset_hound_81_snp_seq.png} &
            \includegraphics[trim=2 0 0 2,clip,width=0.2\columnwidth]{supp_mat/oxford/ground_truth/basset_hound_81_snp2_seq.png} \\
            
            \includegraphics[trim=2 0 0 2,clip,width=0.2\columnwidth]{supp_mat/oxford/ground_truth/saint_bernard_93_reference_img.png} &
            \includegraphics[trim=2 0 0 2,clip,width=0.2\columnwidth]{supp_mat/oxford/ground_truth/saint_bernard_93_our_seq_00.png} & 
            \includegraphics[trim=2 0 0 2,clip,width=0.2\columnwidth]{supp_mat/oxford/ground_truth/saint_bernard_93_pt_seq.png} &
            \includegraphics[trim=2 0 0 2,clip,width=0.2\columnwidth]{supp_mat/oxford/ground_truth/saint_bernard_93_snp_seq.png} &
            \includegraphics[trim=2 0 0 2,clip,width=0.2\columnwidth]{supp_mat/oxford/ground_truth/saint_bernard_93_snp2_seq.png} \\
            
            \includegraphics[trim=2 0 0 2,clip,width=0.2\columnwidth]{supp_mat/ade/ground_truth/ADE_train_00002084_reference_img.png} &
            \includegraphics[trim=2 0 0 2,clip,width=0.2\columnwidth]{supp_mat/ade/ground_truth/ADE_train_00002084_our_seq_00.png} & 
            \includegraphics[trim=2 0 0 2,clip,width=0.2\columnwidth]{supp_mat/ade/ground_truth/ADE_train_00002084_pt_seq.png} &
            \includegraphics[trim=2 0 0 2,clip,width=0.2\columnwidth]{supp_mat/ade/ground_truth/ADE_train_00002084_snp_seq.png} &
            \includegraphics[trim=2 0 0 2,clip,width=0.2\columnwidth]{supp_mat/ade/ground_truth/ADE_train_00002084_snp2_seq.png} \\
            
            \includegraphics[trim=2 0 0 2,clip,width=0.2\columnwidth]{supp_mat/ade/ground_truth/ADE_train_00005219_reference_img.png} &
            \includegraphics[trim=2 0 0 2,clip,width=0.2\columnwidth]{supp_mat/ade/ground_truth/ADE_train_00005219_our_seq_00.png} & 
            \includegraphics[trim=2 0 0 2,clip,width=0.2\columnwidth]{supp_mat/ade/ground_truth/ADE_train_00005219_pt_seq.png} &
            \includegraphics[trim=2 0 0 2,clip,width=0.2\columnwidth]{supp_mat/ade/ground_truth/ADE_train_00005219_snp_seq.png} &
            \includegraphics[trim=2 0 0 2,clip,width=0.2\columnwidth]{supp_mat/ade/ground_truth/ADE_train_00005219_snp2_seq.png} \\
            
            \includegraphics[trim=2 0 0 2,clip,width=0.2\columnwidth]{supp_mat/ade/ground_truth/ADE_train_00009911_reference_img.png} &
            \includegraphics[trim=2 0 0 2,clip,width=0.2\columnwidth]{supp_mat/ade/ground_truth/ADE_train_00009911_our_seq_00.png} & 
            \includegraphics[trim=2 0 0 2,clip,width=0.2\columnwidth]{supp_mat/ade/ground_truth/ADE_train_00009911_pt_seq.png} &
            \includegraphics[trim=2 0 0 2,clip,width=0.2\columnwidth]{supp_mat/ade/ground_truth/ADE_train_00009911_snp_seq.png} &
            \includegraphics[trim=2 0 0 2,clip,width=0.2\columnwidth]{supp_mat/ade/ground_truth/ADE_train_00009911_snp2_seq.png} \\
            
            \includegraphics[trim=2 0 0 2,clip,width=0.2\columnwidth]{supp_mat/ade/ground_truth/ADE_train_00000568_reference_img.png} &
            \includegraphics[trim=2 0 0 2,clip,width=0.2\columnwidth]{supp_mat/ade/ground_truth/ADE_train_00000568_our_seq_00.png} & 
            \includegraphics[trim=2 0 0 2,clip,width=0.2\columnwidth]{supp_mat/ade/ground_truth/ADE_train_00000568_pt_seq.png} &
            \includegraphics[trim=2 0 0 2,clip,width=0.2\columnwidth]{supp_mat/ade/ground_truth/ADE_train_00000568_snp_seq.png} &
            \includegraphics[trim=2 0 0 2,clip,width=0.2\columnwidth]{supp_mat/ade/ground_truth/ADE_train_00000568_snp2_seq.png} \\

    \end{tabular}
    }
    \captionof{figure}{Qualitative comparison of \methodname~with baselines. Given the {\color{blue} context} (blue) strokes, we generate 100 {\color{red} predicted} (red) stroke sequences and plot the one that better matches the {\color{green} ground truth} (green). %Our method produces the sequence closest to the ground truth, suggesting that the distribution of predicted stroke sequences better matches the ground truth
    }
    \label{fig:ground_truth}
\end{table*}
